# Supplementary material for: Language Modeling with Latent Situations
Source: arXiv:2212.10012 source file (2022-12-20)
Supplement: Supplementary file 1 [file 9999_appendix_old.tex]

\label{sec:appendix}
\begin{figure*}
    \centering
    \includegraphics[scale=0.4,trim={0 23cm 33cm 0},clip]{figures/all_domains_errors.pdf}
    \caption{(a) State inference accuracies and (b) sentence prediction accuracies for all 4 domains (TW, TRIP, Recipes, OpenPI). We run the experiments described in \S\ref{sec:state_inference_errors} and \S\ref{sec:sentence_prediction_errors} on the OpenPI domain. Results in OpenPI mirror results in TRIP and Recipes: training explicitly on state does not significantly reduce state inference errors, and states are difficult to use for next sentence prediction (conditioning NSP on state is comparable to conditioning on just the full set of entities alone).}
    \label{fig:all_domains_error_gaps}
\end{figure*}

\section{OpenPI Dataset: State Inference Accuracy \& NSP on Accurate States}
\label{sec:app_openpi}
In addition to the datasets in \S\ref{sec:models_datasets}, we also ran experiments on \textbf{OpenPI}~\cite{tandon-etal-2020-dataset}, which consists of instruction sequences annotated with the changes to entity states that result from executing each instruction. 

As shown in~\cref{fig:all_domains_error_gaps}(a), in OpenPI, similar %
to in TRIP and in Recipes, training with state supervision does not improve state inference accuracy.
For domains where state supervision does not help, state inference is either too difficult, even in the presence of explicit supervision (OpenPI), or too easy and already learned from text-only training (TRIP).

In~\cref{fig:all_domains_error_gaps}(b), it appears that conditioning the LM on states result in more accurate next sentence predictions than conditioning the LM on text in OpenPI. However, this is %
simply %
because the state contains the full set of entities, even unknown ones that have not yet appeared in the prior context.
This is supported by the fact that conditioning the LM on the full set of entities alone results in comparable gains as conditioning on state.
This is a quirk of the contrastive evaluation---the LM simply needs to check whether the entities mentioned in the next sentence matches one of the entities in the state.
Thus, we cannot conclude that the state, in and of itself, is any more informative of the next sentence than the text context.
(It is natural to ask whether this is also the case for TW. However, in TW, we are conditioning on the \textit{current belief state} rather than the full state, which contains only \textit{known facts about known entities}. See more in \S\ref{sec:app_state}.)



\section{Constructing the State}
\label{sec:app_state}
\subsection{State supervision in each domain}
\label{sec:app_state_all_domains}
In each domain, the state is a collection of facts (attributes and/or relations) about each entity.
It is updated each time there is a %
new action, instruction, or sentence.
We convert the state to natural language to take advantage of existing linguistic understanding in pre-trained models. %
Future work can examine the effect of using non-natural-language forms of state.

Below, we discuss the details of this conversion from the available state annotations in each domains.
Sample states from each domain can be found in~\cref{tab:dataset_samples}.

\paragraph{TW}
In TW, the simulator gives us the \textbf{full state}, or the full set of facts describing the state of the world after executing each agent action. Facts are either entity properties (e.g. \texttt{locked(door)}), or relations between two entities (e.g. \texttt{is-in(key, chest)}).
However, since the agent has not explored the full state at the start of each game, at each step, we compute a subset of the facts that the agent \textit{knows about}. We call this the \textbf{belief state}.
We further restrict this subset to only facts that are \textit{causally relevant} to any possible next action that the agent can take, such that all possible next actions can be inferred from just this set. We call this the \textbf{current belief state}. (We explore whether this choice to use different subsets of the state actually matters in \S\ref{sec:app_TW_aux_other_states}).

We compute both these sets heuristically: the belief state consists of all facts about any currently or previously accessible entities that the agent has encountered. %
For the \textit{current} belief state, we discard facts about previously accessible entities and keep only facts about currently accessible entities. Specifically, the current belief state consists of facts about: 1. player location, 2. all currently accessible items (i.e. in the current room or in the inventory), 3. which doorways are accessible from the current room and/or which rooms neighbor the current room.


We convert %
collections of facts to natural language following the same procedure as~\newcite{li-etal-2021-implicit}. Specifically, propositions $p(o)$ are converted to ``\textit{the $\{o\}$ is $\{p\}$}'', while relations $r(o_1,o_2)$ are converted to ``\textit{the $\{o_1\}$ is $\{r\}$ $\{o_2\}$}''.

\paragraph{TRIP}
In TRIP, each sentence of a story is annotated with the %
state changes applied to each of the (up to 15) attributes of that entity. The state annotations take the form of $(\textit{entity}, \textit{attribute}, \textit{value})$ triples.
Each entity attribute is %
associated
with a value indicating the direction of change for that attribute. For example, $(\textit{shirt}, \textit{cleanliness}, \textit{true}\to\textit{false})$ indicates \textit{the shirt became dirty}.

We directly use the provided annotations in TRIP, without filtering for known/causally relevant facts as in TW. 
We do this simply out of ease---TW is synthetically generated, allowing us to hard-code rules for discovering these subsets, while TRIP is real and more complex.
However, note in TRIP that only the relevant entities %
and attributes are annotated, rather than the full state, so the provided annotations %
are already a %
subset of the full state.

Because there are a finite set of (15) attributes and (8) values, we enumerate rules for converting all $(\textit{attribute}, \textit{value})$ pairs to natural language predicates \texttt{VP}. We then convert $(\textit{entity}, \textit{attribute}, \textit{value})$ triples into ``\textit{the $\{$entity$\}$} \texttt{VP}''.


\paragraph{Recipes}
In Recipes, each instruction is annotated with the list of ingredients that have undergone state changes (e.g. \textit{sugar, dough, apples}), and all new states induced by the events in the instruction, given as a list of $(\textit{attribute}, \textit{value})$ pairs (e.g. $(\textit{temperature, hot})$; $(\textit{shape, sliced})$).

Since the provided annotations did not specify which state changes were associated with which entity, we heuristically convert annotations into entity-centric facts by simply assuming all state changes have been applied to all ingredients. Note this can often be a faulty assumption---for example, in~\cref{tab:dataset_samples}, the \texttt{deformed shape} attribute only applies to the chocolate rather than the water.

Finally, we convert these $($\textit{entity}, \textit{attribute}, \textit{value}$)$ triples into natural language descriptions as ``\textit{the $\{$attribute$\}$ of $\{$entity$\}$ is $\{$value$\}$}''. For example, $($\textit{apples}, \textit{shape}, \textit{sliced}$)$ becomes ``\textit{the shape of apples is sliced}''.

\paragraph{OpenPI}
In OpenPI, each instruction is annotated state changes in the form of $($\textit{entity}, \textit{attribute}, \textit{previous value}, \textit{new value}$)$. We convert these to natural language as 
``\textit{the $\{$attribute$\}$ of $\{$\textit{entity}$\}$ is $\{$\textit{new value}$\}$}''. For example, $($\textit{eraser}, \textit{location}, \textit{at store}, \textit{at home}$)$ becomes ``\textit{the location of eraser is at home}''.

\begin{figure*}
    \centering
    \includegraphics[scale=0.34,trim={0 22cm 21cm 0},clip]{figures/all_domains_aux_results.pdf}
    \caption{Training with auxiliary state supervision in TRIP, Recipes, and OpenPI. We vary the total number of examples available, and assume all examples have state annotations. We can see that in all 3 domains, training with auxiliary supervision is unhelpful.}
    \label{fig:NSP_fully_aligned}
\end{figure*}
\section{Additional Results for Auxiliary and Latent State Supervision}
\subsection{Effect of State Supervision on Generation Diversity in TW}
\label{sec:app_TW_diversity}
To measure the diversity of LM outputs, we use \textit{recall} between the set of LM generations and the full set of ground-truth valid sentences. This latter set is provided to us by the TextWorld simulator.
Note that this set is not entirely complete, as there will be generations that are consistent with the \textit{known facts} from the prior context but contradict an \textit{unknown fact}, and is consequently not accepted by the simulator.
However, recall against the simulator-provided set of valid sentences remains a good heuristic for diversity.

We examine how training with auxiliary or latent state supervision affects generation diversity. We use the same models trained in \S\ref{sec:fixing_errors} (with AS and LS on 1000 TW examples paired with varying amounts of state supervision) and evaluate their generation diversity.
Recall from \S\ref{sec:fixing_errors} that both auxiliary and latent state supervision improve coherence.
As shown in~\cref{fig:TW_state_diversity},
neither of them %
reduce diversity to achieve coherence gains. %
However, they do not improve diversity either.
In~\cref{fig:TW_state_diversity}, we train a LM on 1000 examples to predict the next sentence from state. This is plotted as a dotted line.
We can see that a LM that is able to condition on state explicitly produces much more diverse generations, improving recall by over $6$ points. %
It remains an open question as to how to transfer this large diversity improvement to the setting where state annotations are only available at training time.


\subsection{Auxiliary State Supervision in Recipes and OpenPI}
\label{sec:app_aux_train_other}
Results for training with auxiliary state supervision across various data sizes, in the setting where examples are fully aligned with states, is shown in~\cref{fig:NSP_fully_aligned} for Recipes, OpenPI, and TRIP. The analogous TW results can be seen by comparing the blue and red lines in~\cref{fig:TW_choice_of_state}.

In both Recipes and OpenPI, we find similar trends as TRIP: training with auxiliary state \textit{does not} improve generation coherence.
This comes at no surprise given what we found from the state inference accuracy and sentence prediction accuracy experiments in \S\ref{sec:errors_diagnosis} and \S\ref{sec:app_openpi}. State supervision is only useful in domains where state representations are fixable and usable.

\section{T5 Results}
\label{sec:t5_model}
\begin{figure*}
\begin{minipage}[t]{0.56\textwidth}
    \centering
    \includegraphics[scale=0.21,trim={1cm 8cm 34cm 4cm},clip]{figures/T5/state_inference_T5.pdf}
    \caption{Accuracy of states extracted from T5 encoders, using a state probe on a frozen T5 encoder (solid line) vs. a state prediction upper bound where both the T5 encoder and decoder are fine-tuned (dashed line). Analogous to~\cref{fig:state_inference} in main text, with experimental details described in Section~\ref{sec:state_inference_errors}. Note that, as with BART, the possible improvement from directly supervision state representations is large in TW but small in other domains.}
    \label{fig:T5_state_inference}
\end{minipage}
\hfill
\begin{minipage}[t]{0.4\textwidth}
    \centering
    \includegraphics[scale=0.2,trim={1cm 8cm 34cm 4cm},clip]{figures/T5/NSP_state_vs_text_T5.pdf}
    \caption{Next sentence prediction, conditioned on text (solid line) vs. state (dashed line), using the T5 model. Analogous to~\cref{fig:NSP_state_vs_text} in main text, with experimental details described in Section~\ref{sec:sentence_prediction_errors}. Note that, as with BART, conditioning on state only helps in TW.}
    \label{fig:T5_NSP_state_vs_text}
\end{minipage}
\end{figure*}
We rerun the experiments from~\cref{sec:errors_diagnosis} and~\cref{sec:fixing_errors}, but using T5-base~\cite{T5} instead of BART-base. %
We find that T5 gives largely the same results as BART,
where state representations are only inferrable and useful for TW, but not for TRIP (or Recipes; \cref{fig:T5_NSP_state_vs_text,fig:T5_state_inference}),
meaning that training with 
auxiliary and latent 
state supervision gives
gains in generation coherence
for TW, but not for TRIP
(\cref{fig:T5_NSP_partially_aligned}).
In both T5 and BART, 500 TW annotations are sufficient to provide coherence improvements comparable to 9,000 more text-only TW examples.
We find that when using T5 (unlike BART), state supervision also provides significant gains in TW generation \textit{diversity}.
Note that~\cref{fig:T5_NSP_partially_aligned} reports results on only 2 random seeds, thus explaining the higher variance.


\section{Identifying improvable state representations}
\label{sec:errors_diagnosis}
In the idealized generative process of \cref{fig:teaser}, coherence errors can arise in two places: 
in $p(S \mid T)$ (\textbf{state inference errors}) and in $p(T' \mid S)$ (\textbf{sentence prediction errors}).
\citet{li-etal-2021-implicit} found that LMs approximate this generative process by using \emph{context encodings} to represent the state of the world. We thus expect state inference errors to manifest as \emph{encodings from which state representations cannot be extracted}, and prediction errors to manifest as \emph{failure to produce coherent text given ground-truth state representations}.
This section presents an experimental framework for measuring whether each error type is present and correctable in an LM.
\begin{figure}
    \centering
    \includegraphics[scale=0.17,trim={1cm 8cm 34cm 4cm},clip]{figures/state_inference.pdf}
    \vspace{-.5em}
    \caption{Accuracy of states extracted from LM encoders. 
    Solid lines show accuracy of a state \emph{probe} applied to fixed encodings from LMs fine-tuned for text generation with varying amounts of data. 
    Dashed lines show performance of a state prediction \emph{upper bound} in which the encoder and decoder were jointly fine-tuned to predict state representations.
    Shaded areas represent the possible improvement in \emph{state prediction} that could be obtained by directly supervising state representations, which is large for TW but smaller in other domains.
    }
    \label{fig:state_inference}
    \vspace{-1em}
\end{figure}
\subsection{Measuring state inference errors}
\label{sec:state_inference_errors}
\paragraph{Method}

We evaluate the accuracy of (1) models trained to predict states given fixed LM encodings, and (2) upper bound %
models trained to predict states from context text.
The \emph{magnitude} of (1) measures how well LMs encode state, while the \emph{difference} between (2) and (1) measures how much state representations could be improved with additional supervision.
The upper bound is obtained by jointly fine-tuning the encoder and decoder of an LM; the probe is obtained by fine-tuning a decoder only.



\paragraph{Results}
Results are shown in~\cref{fig:state_inference}. 
In TW, we find a large gap between the upper bound and the probe, indicating that states are not well-encoded by models trained on text alone, but 
learnable with targeted supervision.
In TRIP and Recipes, the gap is much smaller. 
In all domains, \textit{simply scaling up the amount of text used to fine-tune the LM does not %
yield improved state representations.}


\subsection{Measuring sentence prediction errors}
\label{sec:sentence_prediction_errors}
\paragraph{Method}
We next evaluate whether, %
in each problem domain, LMs with access to ground-truth state representations can generate more coherent output than LMs that condition on text representations.
We train (1) an $S \to T'$ LM to map from explicit state annotations to next sentences, and (2) a base $T \to T'$ LM. The \emph{magnitude} of (1) measures the prevalence of text prediction errors given an ideal state, while the \emph{difference} between (2) and (1) measures how much generation would in principle be improved by better state representations.

\paragraph{Evaluation}
We use a contrastive evaluation. For each test context $T$ or $S$, models are presented with the true next sentence following the context and (one or more) distractor sentences. We measure the fraction of contexts in which the true next sentence is assigned greater probability than the distractor.



In TW, we select six distractors that \emph{cannot be produced} by the simulator in a given context.
In TRIP, we select a single distractor taken from the implausible story in each pair.
Finally, in Recipes, we use 15 in-batch next sentences as distractors.


\paragraph{Results}

\begin{figure}
    \centering
    \includegraphics[scale=0.17,trim={1cm 8cm 34cm 4cm},clip]{figures/NSP_state_vs_text.pdf}
    \vspace{-.5em}
    \caption{Next sentence prediction, conditioned on text (solid line) vs.\ state (dashed line), across 100-10k text-to-text or state-to-text examples. 
    In TW, ground-truth states improve next-sentence prediction.
    In TRIP and Recipes, models conditioned on state perform \emph{worse}.
    }
    \vspace{-1em}
    \label{fig:NSP_state_vs_text}
\end{figure}

Results are shown in~\cref{fig:NSP_state_vs_text}. In TRIP and Recipes, even ground-truth state representations do not promote more coherent text generation.
In TW, this is reversed, and LMs achieve better performance when conditioning on state.
\\ 

To summarize:
coherence errors in language modeling problems reflect a diverse set of underlying model failures.
In TRIP, states are correctly inferred most of the time, but difficult to use; generation errors arise in next sentence prediction.
In Recipes, states are not correctly inferred and not easily correctable, and also seemingly unhelpful for generation.
In TW, states are incorrectly inferred but inferrable in principle, and useful if inferred. 



\section{Sample LM Generations in TW}
Sample generations from the language model, before and after training with state supervision, can be found in~\cref{tab:LM_samples}.

\section{Infrastructure and Reproduciility}
We ran all experiments on a single 32GB NVIDIA Tesla V100 GPU. We use a BART-base model which has 6 Transformer layers each in its encoder and decoder, and 139M total parameters. Training time varies depending on domain and data size, but generally is not longer than a few hours. As a reference point: on 1000 TW examples, training takes $\sim$1 hour for text-only training, $\sim$1-2 hours for training with auxiliary state supervision, and $\sim$1-3 hours for training with latent state supervision.


\begin{landscape}
\begin{table}[]
    \centering
    \small
    \begin{tabular}{lp{11cm}p{6cm}p{5cm}}
    \toprule
        Dataset & Sample $T$ & Sample $S$ & Sample $T'$ \\
    \midrule
        TW &
        \textit{-= Garage =- \newline [...] You see a locker. You can make out a table. On the table you can make out an American limited edition passkey. There is a closed American limited edition hatch leading west. There is an unblocked exit to the north. \newline > inventory \newline You are carrying nothing. \newline > go north \newline -= Cookhouse =- \newline [...] You make out a case. [...] You see a plate. [...] But oh no! there's nothing on this piece of junk. You hear a noise behind you and spin around, but you can't see anything other than a rack. But oh no! there's nothing on this piece of garbage. You can see a saucepan. The saucepan [...] has nothing on it. [...] You need an unguarded exit? You should try going south. \newline > examine case \newline The case looks strong, and impossible to break. You can't see inside it because the lid's in your way.} &
        \texttt{The plate is in cookhouse} \newline \texttt{The saucepan is in cookhouse} \newline \texttt{The case is in cookhouse} \newline \texttt{The cookhouse is mapped north of garage} \newline \texttt{The rack is in cookhouse} \newline \texttt{The case is closed} \newline \texttt{The garage is mapped south of cookhouse} \newline \texttt{The player is in cookhouse} &
        \textit{> open case} \\
        \\
        
        TRIP &
        \textit{Tom picked up the paper from the copier. \newline Tom picked up the scissors.} &
        \texttt{Tom is conscious} \newline \texttt{The scissors is picked up} \newline \texttt{The scissors are existent} \newline \texttt{The scissors are functional} \newline \texttt{The scissors are moveable} &
        \textit{Tom used the scissors to cut the paper.} \\
        \\
        
        Recipes &
        \textit{Ingredients: chocolate, water, egg white, vanilla, sugar, flour, baking powder, salt, sugar. \newline In large heatproof bowl set over hot water, melt chocolate with water, stirring until smooth.} &
        \texttt{the shape of chocolate is deformed} \newline \texttt{the cookedness of chocolate is cooked} \newline \texttt{the location of chocolate is bowl} \newline \texttt{the temperature of chocolate is hot} \newline \texttt{the shape of water is deformed} \newline \texttt{the cookedness of water is cooked} \newline \texttt{the location of water is bowl} \newline \texttt{the temperature of water is hot} &
        \textit{Remove from heat} \\
        \\
        
        OpenPI &
        \textit{How to spool knit a winter hat. \newline Knit eighty-four inches of flat web. \newline Begin five inches from the end of the web, turn and sew into a rectangular form five inches wide and eight inches long.} &
        \texttt{shape of the webbing is rectangular} \newline \texttt{width of the webbing is wider} \newline \texttt{connection of the ends is unjoined} \newline \texttt{state of ends is loose} \newline \texttt{state of the ends is unattached} \newline \texttt{shape of the yarn is rectangular} \newline \texttt{state of the top is open} &
        \textit{Join the five-inch ends, and draw in the top with the needle and a piece of the material from which the cap was made.} \\
    \bottomrule
    \end{tabular}
    \caption{Sample contexts, states, and next sentences from each domain.}
    \label{tab:dataset_samples}
\end{table}
\end{landscape}

\begin{landscape}
\begin{table}[]
    \centering
    \small
    \begin{tabular}{p{14cm}p{3.5cm}p{5.5cm}}
    \toprule
        Context & 1k Text-only Examples & 1k Text Examples + 500 State Annotations (Latent supervision) \\
    \midrule
        \textit{-= Garage =- \newline [...]
        You see a locker. You can make out a table. On the table you can make out an American limited edition passkey. \newline There is a closed American limited edition hatch leading west. There is an unblocked exit to the north. \newline > inventory \newline You are carrying nothing. \newline [...]
        \newline > go north \newline -= Cookhouse =- \newline [...] 
        You make out a case. There's something strange about this thing being here, but you don't have time to worry about that now. You see a plate. Now why would someone leave that there? The plate is usual. But oh no! there's nothing on this piece of junk. You hear a noise behind you and spin around, but you can't see anything other than a rack. But oh no! there's nothing on this piece of garbage. You can see a saucepan. The saucepan is typical. However, the saucepan, like an empty saucepan, has nothing on it. Hm. Oh well \newline You need an unguarded exit? You should try going south. \newline > examine case \newline The case looks strong, and impossible to break. You can't see inside it because the lid's in your way. \newline [...]}
        & \textit{\textcolor{green}{> examine plate} \newline \textcolor{green}{> examine plate} \newline \textcolor{green}{> examine plate} \newline \textcolor{green}{> examine plate} \newline \textcolor{red}{> open plate}}
        & \textit{\textcolor{green}{> examine plate} \newline \textcolor{green}{> examine plate} \newline \textcolor{green}{> examine plate} \newline \textcolor{green}{> examine plate} \newline \textcolor{red}{> open American limited edition hatch}} \\
    \midrule
        \textit{-= Bar =- \newline [...] %
        You see a box. The box is empty, what a horrible day! You can see a basket. Something scurries by right in the corner of your eye. Probably nothing. You can make out a suitcase. You can see a recliner. But the thing is empty, unfortunately. Were you looking for a mantle? Because look over there, it's a mantle. Looks like someone's already been here and taken everything off it, though. If you haven't noticed it already, there seems to be something there by the wall, it's a bed stand. But the thing is empty. \newline There is a closed type Z door leading west. You don't like doors? Why not try going east, that entranceway is unguarded. \newline > inventory \newline You are carrying nothing. \newline > open basket \newline You open the basket. \newline [...] %
        \newline > go east \newline -= Salon =- \newline [...] %
        As if things weren't amazing enough already, you can even see a portmanteau. Look over there! a couch. Now why would someone leave that there? The couch is normal. On the couch you can see a type Z latchkey. \newline There is an exit to the west. Don't worry, it is unblocked. \newline [...] \newline %
        > examine portmanteau \newline The portmanteau looks strong, and impossible to destroy. You can't see inside it because the lid's in your way. \newline [...] %
        \newline > open portmanteau \newline You open the portmanteau.}
        & \textit{\textcolor{green}{> go west} \newline \textcolor{green}{> go west} \newline \textcolor{green}{> examine couch} \newline \textcolor{red}{> examine bed stand} \newline \textcolor{red}{> examine bed stand}}
        & \textit{\textcolor{green}{> go west} \newline \textcolor{green}{> go west} \newline \textcolor{green}{> examine couch} \newline \textcolor{red}{> examine suitcase} \newline \textcolor{green}{> take type Z latchkey from couch}}  \\
        
    \bottomrule
    \end{tabular}
    \caption{LM generations in TW, before and after training with state supervision. We take five samples from each LM for each context. \textcolor{green}{Green} indicates coherent generations. \textcolor{red}{Red} indicates incoherent generations.} %
    \label{tab:LM_samples}
\end{table}
\end{landscape}
